# Supplementary material for: Unusual Nonmagnetic Ordered State in CeCoSi Revealed by $^{59}$Co-NMR and NQR Measurements
Source: arXiv:2101.06830 source file (2021-01-18)
Supplement: Supplementary file 1 [file supplemental.pdf]

# Supplemental Materials for
# "Unusual Nonmagnetic Ordered State in CeCoSi Revealed by $^{59}$Co-NMR and NQR Measurements"

Masahiro Manago, Hisashi Kotegawa, Hideki Tou, and Hisatomo Harima
*Department of Physics, Kobe University, Kobe, Hyogo 657-8501, Japan*

Hiroshi Tanida
*Liberal Arts and Sciences, Toyama Prefectural University, Imizu, Toyama 939-0398, Japan*

## I. NMR KNIGHT SHIFT AT AMBIENT PRESSURE

When the magnetic field is applied to the system, the nucleus feels the internal field created by the electrons through the hyperfine interaction in addition to the applied field. This internal field is usually expressed as the dimensionless Knight shift tensor $K$, and the total magnetic field is $\boldsymbol{H}_{\rm tot} = (1+K)\boldsymbol{H}_0$, where the $\boldsymbol{H}_0$ represents the applied field. The form of the Knight shift tensor is restricted by the local symmetry of the nucleus. In the case of the Co site in the non-ordered state in CeCoSi, the Knight shift at the Co site is the form of

$$K = \begin{pmatrix} K_{aa} & 0 & 0 \\ 0 & K_{aa} & 0 \\ 0 & 0 & K_{cc} \end{pmatrix}, \quad (1)$$

where the $c$ represent the [001] direction, because of the $\bar{4}m2$ local tetragonal symmetry. The measurements with $H \parallel [100]$ and [001] give the full information of the Knight shift tensor in the non-ordered state above $T_0$.

Because the $^{59}$Co nucleus ($I = 7/2$, nuclear gyromagnetic ratio $\gamma_{\rm n}/2\pi = 10.03$ MHz/T, and electric quadrupole moment $Q = 0.42 \times 10^{-28}$ m$^2$ [2, 3]) interacts with the electric field gradient of the atomic site, the NMR spectra splits into seven

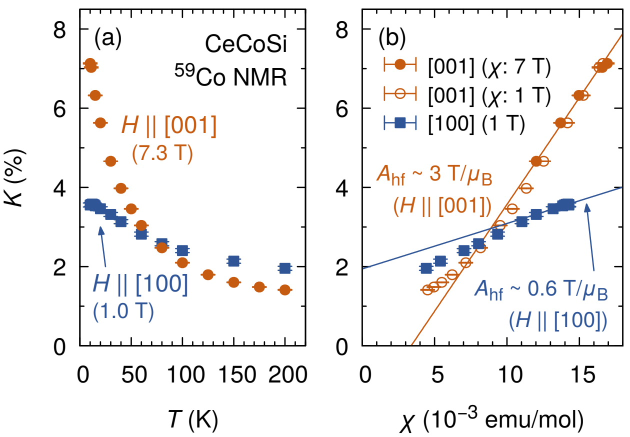


FIG. 1. (a) $^{59}$Co NMR Knight shift in CeCoSi at ambient pressure with the field along the [100] (at 1 T) and [001] (at 7.3 T) directions above $T_{\rm N}$. (b) The relation between $\chi$ and $K$ with temperatures as an implicit parameter ($K$–$\chi$ plot). The susceptibility is from Ref. 1. For the [001] direction, the susceptibility results are shown for the 1 and 7 T. The hyperfine coupling constant $A_{\rm hf}$ was deduced from the linear fit of the $K$ values against the $\chi$ below 30 K.

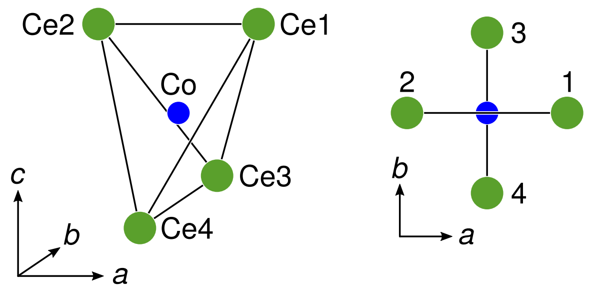


FIG. 2. Left: The Co atom and the four nearest Ce atoms forming a tetrahedron. The smaller and the larger balls indicate Co and Ce atoms, respectively. Right: Top view of the left panel. The Ce atoms do not locate at the same plane.

($2I$) lines. The value of the $^{59}$Co Knight shift was extracted from the frequency of the central peak the seven quadrupole split spectra. The effect of the quadruple shift was subtracted by numerical diagonalization of the total nuclear Hamiltonian. Figure 1(a) shows the $^{59}$Co NMR Knight shift along the [100] and [001] directions in the single-crystalline CeCoSi sample at ambient pressure. The sample direction was aligned by eye, and the misalignment of the field is typically an order of $\sim 5^\circ$. The Knight shift increased as the temperature gets lower, as observed in the macroscopic susceptibility [1, 4]; however, contrary to the almost isotropic susceptibility, the Knight-shift value is about 2 times larger for [001] directions than that of [100] just above $T_{\rm N}$. Figure 1(b) shows the relation between the susceptibility $\chi$ and the Knight shift $K$ with the temperature as an implicit parameter (the $K$–$\chi$ plot). The susceptibility was referred from Ref. 1. The relation $K = A_{\rm hf}\chi + K_0$ roughly holds for these directions. The kink in the $K$–$\chi$ plot is seen at 60–100 K depending on the directions, and it is probably due to the crystal electric field effect. The estimated hyperfine coupling constants are $A^a_{\rm hf} \sim 0.6$ T/$\mu_{\rm B}$ for the [100] and $A^c_{\rm hf} \sim 3$ T/$\mu_{\rm B}$ for the [001] direction. The experimental results below 30 K were used for analyzing $A_{\rm hf}$ values.

## II. HYPERFINE COUPLING BETWEEN THE Co NUCLEUS AND 4$f$ ELECTRONS

Here we present the symmetry consideration of the hyperfine coupling tensor of the Co site. The Co site is surrounded by four Ce atoms, which form a tetrahedron, as shown in Fig. 2. The internal field at the Co site created by these nearest Ce

moments are written as

$$\boldsymbol{H}_{\rm int} = \sum_{i=1}^{4} \boldsymbol{B}_i \cdot \boldsymbol{m}_i, \tag{2}$$

where $\boldsymbol{B}_i$ is the coupling tensor between $i$ site and $\boldsymbol{m}_i$ is the magnetic moment of the $i$ site. The structure of $\boldsymbol{B}_i$ and the relation between different $i$ sites are restricted by the crystallographic symmetry. In the state above $T_0$, the crystal structure is tetragonal $P4/nmm$, and the Co site is located at the $\bar{4}m2$ site. This leads to

$$\boldsymbol{B}_1 = \begin{pmatrix} B_{aa} & 0 & B_{ac} \\ 0 & B_{bb} & 0 \\ B_{ca} & 0 & B_{cc} \end{pmatrix} \tag{3}$$

for the site 1. Then, the site 2 in the same $z$ plane as 1 satisfies

$$\boldsymbol{B}_2 = \begin{pmatrix} B_{aa} & 0 & -B_{ac} \\ 0 & B_{bb} & 0 \\ -B_{ca} & 0 & B_{cc} \end{pmatrix} \tag{4}$$

because the site 2 is connected to the site 1 through the $C_2$ rotation with respect to the $z$ axis. The site 3 and 4 are connected to the site 1 and 2 through the $S_4$ operation, leading to

$$\boldsymbol{B}_3 = \begin{pmatrix} B_{bb} & 0 & 0 \\ 0 & B_{aa} & -B_{ac} \\ 0 & -B_{ca} & B_{cc} \end{pmatrix}, \quad \boldsymbol{B}_4 = \begin{pmatrix} B_{bb} & 0 & 0 \\ 0 & B_{aa} & B_{ac} \\ 0 & B_{ca} & B_{cc} \end{pmatrix}. \tag{5}$$

In the state above $T_0$, all the Ce moments point to the same direction, and thus, the internal field at the Co site is

$$\boldsymbol{H}_{\rm int} = (\boldsymbol{B}_1 + \boldsymbol{B}_2 + \boldsymbol{B}_3 + \boldsymbol{B}_4) \cdot \boldsymbol{m} \tag{6}$$

$$= \begin{pmatrix} 2(B_{aa} + B_{bb}) & 0 & 0 \\ 0 & 2(B_{aa} + B_{bb}) & 0 \\ 0 & 0 & 4B_{cc} \end{pmatrix} \cdot \boldsymbol{m} \tag{7}$$

$$\equiv \begin{pmatrix} A^a_{\rm hf} & 0 & 0 \\ 0 & A^a_{\rm hf} & 0 \\ 0 & 0 & A^c_{\rm hf} \end{pmatrix} \cdot \boldsymbol{m}. \tag{8}$$

The microscopic hyperfine coupling constants $B_{ij}$ are related to $A^a_{\rm hf}$ and $A^c_{\rm hf}$ introduced in the previous section.

If the $\boldsymbol{q} = \boldsymbol{0}$ AFM ordering occurs, the moments satisfies $\boldsymbol{m}_1 = \boldsymbol{m}_2 = -\boldsymbol{m}_3 = -\boldsymbol{m}_4 \equiv \boldsymbol{m}_{\rm AFM}$, and the internal field is

$$\boldsymbol{H}_{\rm int} = (\boldsymbol{B}_1 + \boldsymbol{B}_2 - \boldsymbol{B}_3 - \boldsymbol{B}_4) \cdot \boldsymbol{m}_{\rm AFM} \tag{9}$$

$$= \begin{pmatrix} 2(B_{aa} - B_{bb}) & 0 & 0 \\ 0 & -2(B_{aa} - B_{bb}) & 0 \\ 0 & 0 & 0 \end{pmatrix} \cdot \boldsymbol{m}_{\rm AFM}. \tag{10}$$

The staggered component along the $z$ axis is cancelled at the Co site, and especially, the internal field is absent when $\boldsymbol{m}_{\rm AFM} \parallel$ [001]. Therefore, it is unusual that the NMR line splits with an induced field along the [001] direction below $T_0$.

If the $\boldsymbol{q} = \boldsymbol{0}$ AFM causes orthorhombic distortion, the relation of $\boldsymbol{B}_i$ between different Ce sites can be altered. For instance, the distortion along the [100] direction breaks the relation between the pairs of (1,2) and (3,4) sites, leading

$$\boldsymbol{H}_{\rm int} = (\boldsymbol{B}_1 + \boldsymbol{B}_2 - \boldsymbol{B}'_3 - \boldsymbol{B}'_4) \cdot \boldsymbol{m}_{\rm AFM} \tag{11}$$

$$= \begin{pmatrix} 2(B_{aa} - B'_{bb}) & 0 & 0 \\ 0 & -2(B'_{aa} - B_{bb}) & 0 \\ 0 & 0 & 2(B_{cc} - B'_{cc}) \end{pmatrix} \cdot \boldsymbol{m}_{\rm AFM}. \tag{12}$$

The internal field along the [001] direction is possible if the staggered moments tilt from the [001] plane.

If the AFM state is not limited to $\boldsymbol{q} = \boldsymbol{0}$, the internal field can emerge along the [001] direction, although such a magnetic structure is inconsistent with the ordered state below $T_0$. For instance, in the checkerboard structure with $\boldsymbol{q} = (\pi/a, \pi/a, 0)$ ($a$ is the lattice constant), the moments satisfy $\boldsymbol{m}_1 = -\boldsymbol{m}_2 = \boldsymbol{m}_3 = -\boldsymbol{m}_4 \equiv \boldsymbol{m}_{\rm AFM}$. The internal field is

$$\boldsymbol{H}_{\rm int} = (\boldsymbol{B}_1 - \boldsymbol{B}_2 + \boldsymbol{B}_3 - \boldsymbol{B}_4) \cdot \boldsymbol{m}_{\rm AFM} \tag{13}$$

$$= \begin{pmatrix} 0 & 0 & 2B_{ac} \\ 0 & 0 & 2B_{ac} \\ 2B_{ca} & 2B_{ca} & 0 \end{pmatrix} \cdot \boldsymbol{m}_{\rm AFM}. \tag{14}$$

The internal field along the [001] direction is induced when the $\boldsymbol{m}_{\rm AFM}$ lies in the plane.

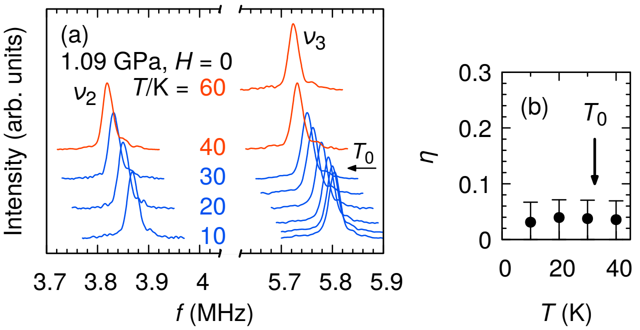


FIG. 3. (a) $^{59}$Co NQR spectra without a field at 1.09 GPa in CeCoSi. (b) The temperature dependence of the asymmetric parameter $\eta$ at 1.09 GPa deduced from the NQR frequencies shown in (a).

## III. EXAMINATION OF THE TETRAGONAL SYMMETRY BELOW $T_0$ BY NQR

We examined whether the tetragonal symmetry at the Co site is preserved below $T_0$ or not using the $^{59}$Co NQR spectra. The nuclear-spin Hamiltonian without the magnetic field is

$$\mathcal{H}_{\rm Q} = \frac{\hbar\omega_{\rm Q}}{6}\left\{\left[3I_z^2 - I(I+1)\right] + \frac{1}{2}\eta(I_+^2 + I_-^2)\right\}, \tag{15}$$

where $\omega_{\rm Q}$ is the quadrupole frequency, $\eta$ is the asymmetric parameter. The coordinate in the above equation is chosen so that the electronic field gradient at the nuclear site ($V_{ij}$) is diagonalized and satisfies the relation $|V_{zz}| \geq |V_{yy}| \geq |V_{xx}|$. The $\omega_{\rm Q}$ is proportional to $V_{zz}$ along the [001] axis (the maximum

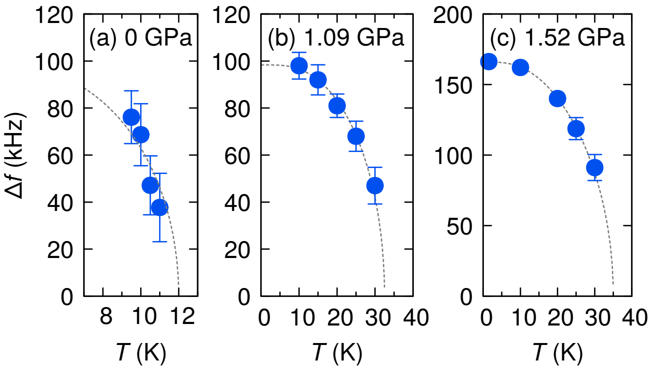


FIG. 4. (a–c) Temperature dependence of the split width $\Delta f$ of the $^{59}$Co NMR lines below $T_0$ at (a) 0, (b) 1.09, and (c) 1.52 GPa. The dashed lines indicate the temperature evolution of the BCS-type order parameter. Parameters of the curve at 0 GPa were given by hand, while the results at 1.09 and 1.52 GPa were obtained by a least-square method.

principal axis), and the asymmetric parameter is $\eta = |V_{xx} - V_{yy}|/|V_{zz}|$ and satisfies $0 \leq \eta \leq 1$.

In the case of the $^{59}$Co ($I = 7/2$) site in CeCoSi above $T_0$, $\eta = 0$ by the local symmetry $\bar{4}m2$ ($\bar{4}$ is the sufficient condition for $\eta = 0$) and the $z$ axis is the [001] direction. Then, the three NQR lines arise from the $\pm m \leftrightarrow \pm(m+1)$ ($m = 1/2,\ 3/2$, and $5/2$) level transitions with the resonant frequencies $\nu_i = i\nu_{\mathrm{Q}}$ ($i \equiv m + 1/2 = 1, 2, 3$), where $\nu_{\mathrm{Q}} \equiv \omega_{\mathrm{Q}}/(2\pi)$.

If the $\bar{4}$ symmetry of the Co is lost below $T_0$, $\eta$ gets a nonzero value, and the frequency $\nu_i$ no longer has an integer ratio. Within the second-order perturbation theory with respect to the $\eta$ term, the ratio between $\nu_2$ and $\nu_3$ for the $I = 7/2$ nuclei is

$$\frac{\nu_3}{\nu_2} = \frac{3}{2} + \frac{7}{10}\eta^2. \tag{16}$$

Thus, measurements of the (at least) two NQR lines enable us to examine whether the tetragonal symmetry is broken or not at the Co site. NMR spectra with a magnetic field is more sensitive to the emergence of a small $\eta$ in general; however, we chose the NQR spectra to find $\eta$ this time because anomalous splitting occurs with applying field below $T_0$ in NMR, which makes the deduction of $\eta$ difficult.

Figure 3(a) shows the part of the $^{59}$Co NQR spectra at the $\nu_2$ and $\nu_3$ lines at 1.09 GPa. The obtained asymmetric parameter $\eta$ is shown in Fig. 3(b). The value of $\eta$ remains almost zero below $T_0 \simeq 33$ K, meaning that the breaking of the tetragonal symmetry at the Co site was not detected by the NQR spectra. Although we cannot exclude the possibility that the tetragonal symmetry is broken with a nonzero $\eta$ below the detection limit, it is more likely that CeCoSi remains tetragonal because the phase transition at $T_0$ was clearly detected in the $\nu_{\mathrm{Q}}$.

## IV. ANALYSIS OF THE NMR SPLIT DISTANCE

Figures 4(a–c) show the temperature dependence of the NMR split distance at 0, 1.09, and 1.52 GPa. The distance $\Delta f$, or the difference of the two peaks in frequency, monotonically increases below $T_0$. These results are consistent with the second-order transition. We tentatively adopt the BCS-type temperature evolution of the order parameter to reproduce $\Delta f$ assuming that it is proportional to the order parameter. We used an approximate function of the order parameter to reproduce the experiments:

$$\Delta f(T) = \Delta f_0 \tanh\left[a(T_{\mathrm{c}}/T - 1)^{1/2}\right], \tag{17}$$

where $\Delta f_0$ and $a$ are fitting parameters. The results are shown with the dashed lines. The theoretical curves were roughly in agreement with the experiments.

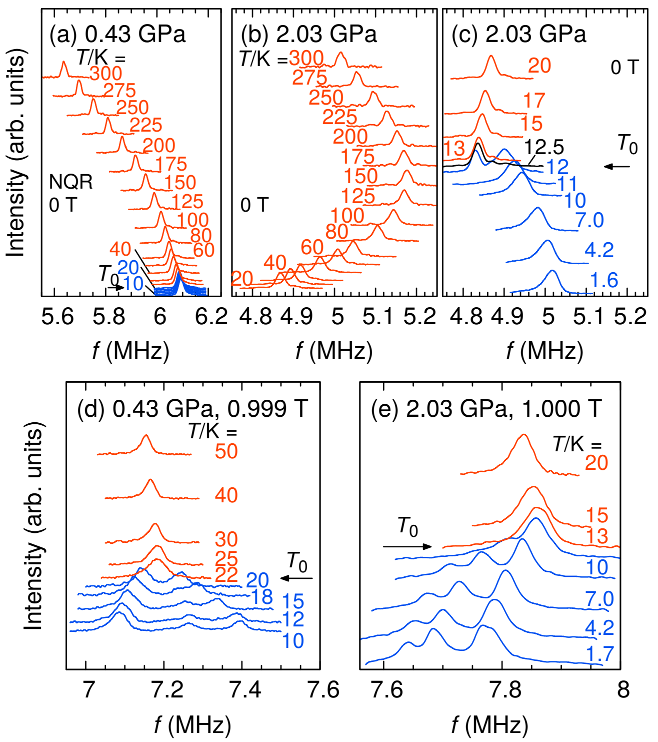


FIG. 5. (a–c) $^{59}$Co NQR spectra without an external field at (a) 0.43 and (b,c) 2.03 GPa in CeCoSi. (d,e) The NMR spectra at (d) 0.43 and (e) 2.03 GPa under the field of $\mu_0 H = 1$ T. The field angle was $\theta \sim 85°$ at these pressures.

## V. NMR AND NQR SPECTRA AT 0.43 AND 2.03 GPa

Figures 5(a–c) show the NQR spectra at 0.43 and 2.03 GPa. The kink is clearer at 2.03 GPa than at 0.43 GPa, and the $\nu_{\mathrm{Q}}(T)$ gets a maximum at 2.03 GPa.

Figures 5(d,e) show the NMR spectra at 0.43 and 2.03 GPa under the field of 1 T with the angle $\theta \sim 85°$. The spectra started to split at $T_0$ in these pressures, indicating the symmetry reduction. The number of peaks is three in these cases. We performed measurements in the order of 1.09, 1.52, 2.03, and 0.43 GPa. Three peaks were remarkably observed in the last two pressures. We suspect the possibility that the sample may be damaged by the successive application of pressure. It is

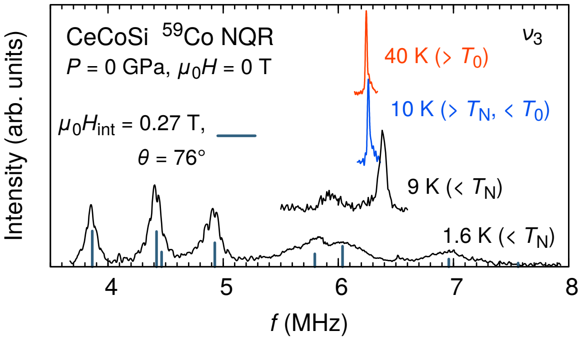


FIG. 6. ${}^{59}$Co NQR spectra without an external field at ambient pressure in several temperatures in CeCoSi. The spectra are shifted vertically. The vertical lines for the result at 1.6 K are the calculated result with the internal field of 0.27 T and the angle 76° from the [001] axis.

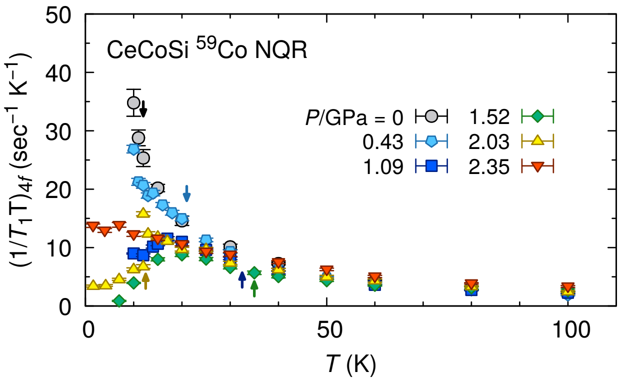


FIG. 7. Temperature dependence of ${}^{59}$Co NQR nuclear spin-lattice relaxation rate divided by temperature $1/T_1T$ of CeCoSi from the Ce-$4f$ electrons. The vertical arrows indicate $T_0$.

a future task to confirm whether more than two peaks is an intrinsic phenomenon or not.

## VI. NQR SPECTRA IN THE ANTIFERROMAGNETIC STATE

We measured the NQR (zero-field NMR) spectrum in the antiferromagnetic (AFM) state at ambient pressure to get information about the magnetic structure. Figure 6 shows the spectra at 9 and 1.6 K below $T_N$ at ambient pressure in addition to the results above $T_N$. The NQR spectrum started to split at 9 K and showed a complicated structure with many peaks because of the internal field in the AFM state. The simulated spectra are shown with vertical lines in Fig. 6. The best fit of the experiments was obtained with the internal field $\mu_0 H_{int} = 0.27$ T and the field angle $\theta = 76°$ from the [001] axis at the Co site. The Co site remains one site below $T_N$. This result indicates the commensurate AFM structure, and is consistent with the polarized neutron scattering measurement [5]. Although the neutron experiment indicates that the Ce moment is parallel to the [100] direction, our data suggests that the Ce moments slightly tilt to the [001] direction, which makes the $\theta < 90°$, i.e., the emergence of the internal field along the [001] direction at the Co site. This is possible because of the orthorhombic distortion of the crystal, as mentioned above. The tilt of the Ce moment is consistent with the susceptibility drop at $T_N$ in the [001] direction as well as in the [100] [1].

## VII. NUCLEAR SPIN-LATTICE RELAXATION RATE $1/T_1$

Figure 7 shows the ${}^{59}$Co nuclear spin-lattice relaxation rate $1/T_1$ divided by temperature $1/T_1T$ in CeCoSi. The Co $3d$ part was subtracted using the results of LaCoSi. $1/T_1$ can detect the magnetic fluctuations perpendicular to the maximum principal axis of the electric field gradient ([001] axis in the Co site). $1/T_1T$ increases as the temperature decreases much above $T_0$ in any pressure, reflecting the localized nature of the $4f$ electrons. $1/T_1T$ showed a critical magnetic fluctuations around $T_N$ at ambient pressure. However, the divergence of $1/T_1T$ was suppressed at 1.09 GPa. The stabilization of the ordered phase below $T_0$ may be related to this suppression, as discussed in the main text.

## VIII. LIST OF POSSIBLE SPACE GROUPS BELOW $T_0$

Details of the possible space groups below $T_0$ are shown in Tab. I [6]. The maximal subgroups of the No. 129 ($P4/nmm$) without superstructure are chosen. The No. 129 is a primitive tetragonal group, and 16 symmetry operations belong to this group. In the maximal subgroups, 8 symmetry operations remain. There is an orthorhombic space group (No. 59), and the others are tetragonal. Because the unit cell volume does not change across the transition for these groups, the multiplicity of the atom should be preserved. In some space groups, Ce or Co sites split into two inequivalent sites. The No. 85 and No. 113 are consistent with our NQR results, as discussed in the main text. The atomic positions do not need to shift, i.e., the notation of the coordinate remains unchanged, across the transition to the space groups No. 85 and No. 113.

TABLE I. Possible space groups for the ordered state below $T_0$ in CeCoSi. The Wyckoff letter and the site symmetry of the atoms are shown for each space group. The atomic position is shown when the notation changes or the atomic position splits. The first row shows the space group No. 129 in the room-temperature state in the origin choice 1. The apparent shift of the positions in No. 99 is due to the change of the origin.

| Space group | Ce site | Co site | Si site |
|---|---|---|---|
| No. 129 $P4/nmm$ | $2c$ $4mm$ $(0,1/2,z)$, $(1/2,0,\bar{z})$ | $2a$ $\bar{4}m2$ $(0,0,0)$, $(1/2,1/2,0)$ | $2c$ $4mm$ $(0,1/2,z)$, $(1/2,0,\bar{z})$ |
| No. 59 $Pmmn$ | $2a$ $mm2$ | $2b$ $mm2$ | $2a$ $mm2$ |
| No. 85 $P4/n$ | $2c$ $4..$ | $2a$ $\bar{4}..$ | $2c$ $4..$ |
| No. 90 $P42_12$ | $2c$ $4..$ | $2a$ $2.22$ | $2c$ $4..$ |
| No. 99 $P4mm$ | $1a$ $4mm$ $(0,0,z)$; $1b$ $4mm$ $(1/2,1/2,z')$ | $2c$ $2mm.$ $(1/2,0,z)$, $(0,1/2,z)$ | $1a$ $4mm$ $(0,0,z)$; $1b$ $4mm$ $(1/2,1/2,z')$ |
| No. 113 $P\bar{4}2_1m$ | $2c$ $2.mm$ | $2a$ $\bar{4}..$ | $2c$ $2.mm$ |
| No. 115 $P\bar{4}m2$ | $2g$ $2mm.$ | $1a$ $\bar{4}m2$ $(0,0,0)$; $1b$ $\bar{4}m2$ $(1/2,1/2,0)$ | $2g$ $2mm.$ |


[1] H. Tanida, K. Mitsumoto, Y. Muro, T. Fukuhara, Y. Kawamura, A. Kondo, K. Kindo, Y. Matsumoto, T. Namiki, T. Kuwai, and T. Matsumura, Successive phase transition at ambient pressure in CeCoSi: Single crystal studies, J. Phys. Soc. Jpn. **88**, 054716 (2019).

[2] G. C. Carter, L. H. Bennett, and D. J. Kahan, *Metallic Shifts in NMR* (Pergamon press, New York, 1977).

[3] J. R. de Laeter, J. K. Böhlke, P. De Bièvre, H. Hidaka, H. S. Peiser, K. J. R. Rosman, and P. D. P. Taylor, Atomic weights of the elements. review 2000 (iupac technical report), Pure Appl. Chem. **75**, 683 (2003).

[4] E. Lengyel, M. Nicklas, N. Caroca-Canales, and C. Geibel, Temperature-pressure phase diagram of CeCoSi: Pressure-induced high-temperature phase, Phys. Rev. B **88**, 155137 (2013).

[5] S. E. Nikitin, D. G. Franco, J. Kwon, R. Bewley, A. Podlesnyak, A. Hoser, M. M. Koza, C. Geibel, and O. Stockert, Gradual pressure-induced enhancement of magnon excitations in CeCoSi, Phys. Rev. B **101**, 214426 (2020).

[6] T. Hahn, ed., *International tables for crystallography*, 5th ed., Vol. A (Springer, 2005) corrected reprint of the 5th edition.
